# Supplementary material for: Fast 3D cell tracking with wide-field fluorescence microscopy through deep learning
Source: arXiv:1805.05139 ancillary file (2018-05-15)
Supplement: Supplementary file 1 [file Supplement.pdf]

# Fast 3D cell tracking with wide-field fluorescence microscopy through deep learning: supplementary material

Kan Liu[2,†], Hui Qiao[1,†], Jiamin Wu[1],
Haoqian Wang[3], Lu Fang[2], Qionghai Dai[1,2,*]

[1] Department of Automation, Tsinghua University, China
[2] Tsinghua-Berkeley Shenzhen Institute, Tsinghua University, China
[3] Graduate School at Shenzhen, Tsinghua University, China

[*] Corresponding author: qhdai@tsinghua.edu.cn

May 14, 2018

## 1 Neural Network Architecture Details

The schematic architectures of our convolutional neural networks (CNNs) are illustrated in Fig. 1. Both architectures consist of several functional layers: convolution layer, pooling layer, fully connected layer, and output layer. The first 5 stages (denoted as ”Layer”) are composed of convolutional layers and pooling layers. In each ”Layer”, a convolutional layer (depicted as a green block) with the rectified linear unit (ReLU) extracts feature maps from the previous layer, and then a pooling layer (depicted as a blue block) downsamples the feature maps before the next convolution layer. We increase the number of features learned in each ”Layer” by gradually increasing the number of channels for high level feature inference. The size of all the kernels (filters) throughout the convolutional layers is $3 \times 3$. For the final classification, the extracted feature representation of ”Layer 5” is fed into the fully connected layers (denoted as ”FC1” and ”FC2”), and the output layer gives a predicted response.

The input of lateral detection CNN is a $128 \times 128$-pixel patch cropped from the raw wide-field fluorescence image and the output is a binary response ($\hat{y} = \pm 1$). The positive value means there exist diffraction patterns at the central $x$-$y$ (lateral) position of the input image while the negative value is opposite. Regarding to the axial localization CNN, we focus on the predicted positive samples of lateral detection CNN and the output is a $50$-element vector ($\hat{z}_1$ to $\hat{z}_{50}$). Each element, having a probability value between 0 and 1, represents an axial position and the whole vector covers an axial range from the focal plane to $100$ microns above with 2-micron spacing. To be specific, the positive element (higher than 0.5) indicates that there is a fluorescent probe locating at

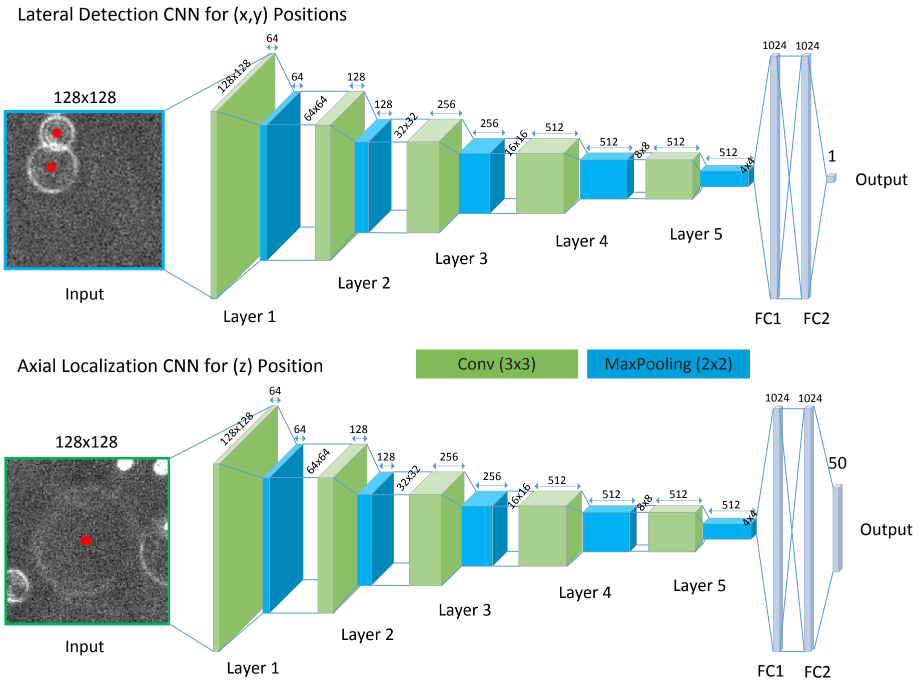


Figure 1: Detailed schematic architectures of our CNNs, indicating the number of layers and nodes. The filter sizes of convolution (Conv) and max pooling (MaxPooling) are $3 \times 3$ and $2 \times 2$, respectively.

the represented axial position while the negative element (lower than 0.5) is opposite. Based on this multi-label design, axial localization CNN makes it possible to simultaneously recognize the different axial positions of multiple diffraction patterns that have the same lateral position.

## 2 Network Training

The randomly selected training samples for our convolutional neural networks are shown in Fig. 2. During the training procedure, we choose the hinge loss [1] for lateral detection CNN as

$$L_1(\hat{y}, y) = \max\{0, 1 - \hat{y}y\}, \tag{1}$$

where $\hat{y}$ is the estimated output and $y$ is the corresponding true label, and the cross-entropy loss [2] for axial localization CNN given by

$$L_2(\hat{z}, z) = -\sum_{i=1}^{50}(z_i \log(\hat{z}_i) + (1 - z_i)\log(1 - \hat{z}_i)), \tag{2}$$

where $\hat{z}$ is the estimated output and $z$ is the corresponding true label.

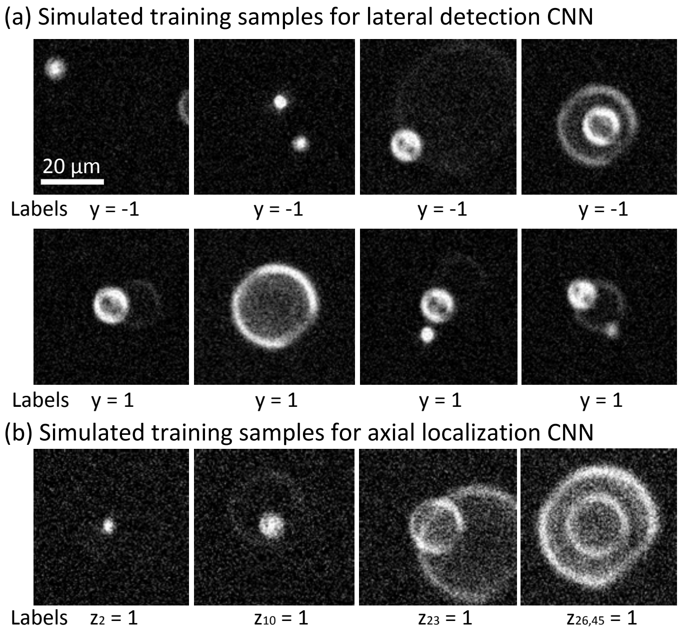


Figure 2: Simulated training samples for our CNNs.

# 3 Network testing

After finishing the training process, the trained CNNs can perform 3D localization without any priori knowledge. To numerically evaluate the performance of our method, we tested it with a localization experiment of 1 ul fluorescent beads (1 μm, type F10002) uniformly immersed into 10 ml agarose. Given the captured epifluorescence image, the trained networks took about 1 minute to obtain the 3D localization result in a volume of $200 \times 200 \times 100$ $\mu m^3$. As shown in Fig. 3, the ground truth (GT) positions of the beads were retrieved from a deconvolved wide-field focal stack of the same agarose volume.

# 4 Fast 3D tracking of multiple objects

The accurate localization of multiple objects in 3D by a single wide-field fluorescence image facilitates fast 3D tracking of multiple objects with a normal microscope. For verification, we first conducted several experiments on zebrafish to track the 3D movement of multiple blood cells. The size of the tagged fluorophore in a blood cell was about 5 μm, leading to a different diffraction pattern from the bead. To improve the localization accuracy, we recorded a new focal stack of a zebrafish blood cell to synthesize sufficient samples for the network training, as shown in Fig. 4. In addition to the 100-fps experiment of the blood cells tracking in zebrafish, we did another experiment with a slower blood flow and the video was captured at 30 fps. The localization re-

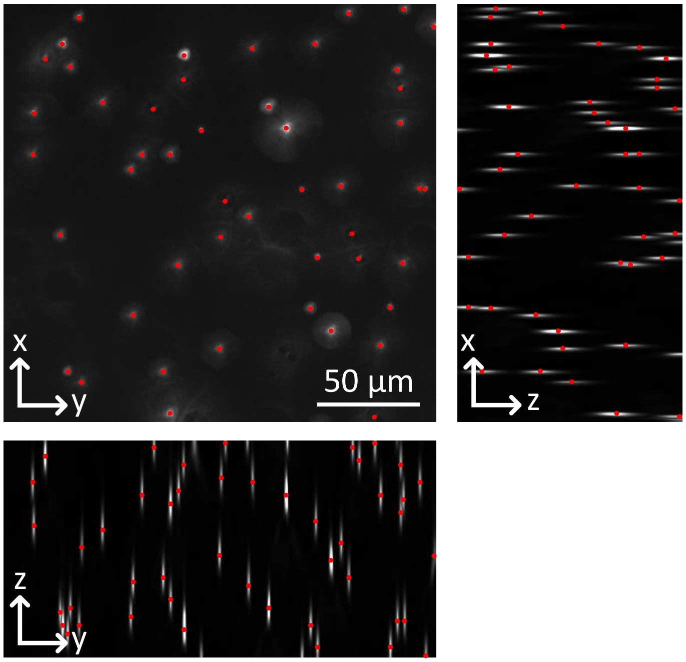


Figure 3: Maximum-intensity projection of a deconvolved wide-field focal stack. The sample consists of 1-μm fluorescent beads (marked by red spots) in agarose.

sults of three different time stamps by our method and maximum likelihood estimation (MLE) method are illustrated in Fig. 5(a). More cells can be detected by our method, especially for cells at the deeper region with lower contrast, due to the higher robustness of our method. The comparison of the tracking traces is also shown in Fig. 5(b) with a much larger axial range in the results of our method.

Since it's hard to get the ground truth of the experimental 3D traces of the blood cells for comparison, we performed a simulated tracking experiments for detailed analysis of the tracking accuracy in several different conditions, as shown in Fig. 6. We randomly placed 16 1-μm fluorescent beads in the volume of $100 \times 100 \times 100$ $\mu m^3$. Then we simulated the movement of these beads in lateral dimension (Fig. 6(a)) and axial dimension (Fig. 6(b)), respectively. Although both of the algorithms work well in sparse region with the Kalman-filter-based tracking algorithm, our proposed method has much better results in the regions of dense cells owing to the higher localization accuracy and the stronger ability of demixing multiple objects. In addition, a test of the beads with random movement is also demonstrated in Fig. 6(c) to show the uniform performance in 3D of our method.

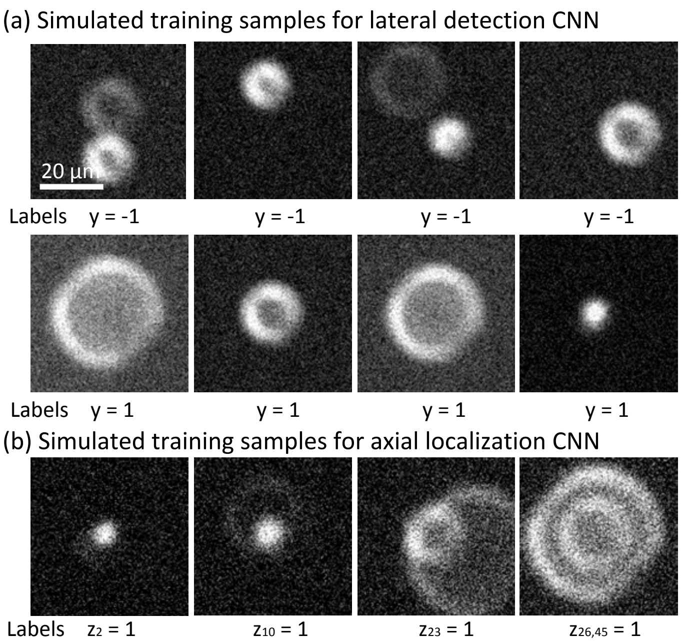


Figure 4: Simulated training samples for CNNs to perform 3D localization of zebrafish blood cells.

# References


[1] K. Chatfield, K. Simonyan, A. Vedaldi, and A. Zisserman, "Return of the devil in the details: Delving deep into convolutional nets," arXiv:1405.3531 (2014).

[2] O. Ronneberger, P. Fischer, and T. Brox, "U-net: Convolutional networks for biomedical image segmentation," in *International Conference on Medical Image Computing and Computer-assisted Intervention* (Springer, 2015), pp. 234–241.

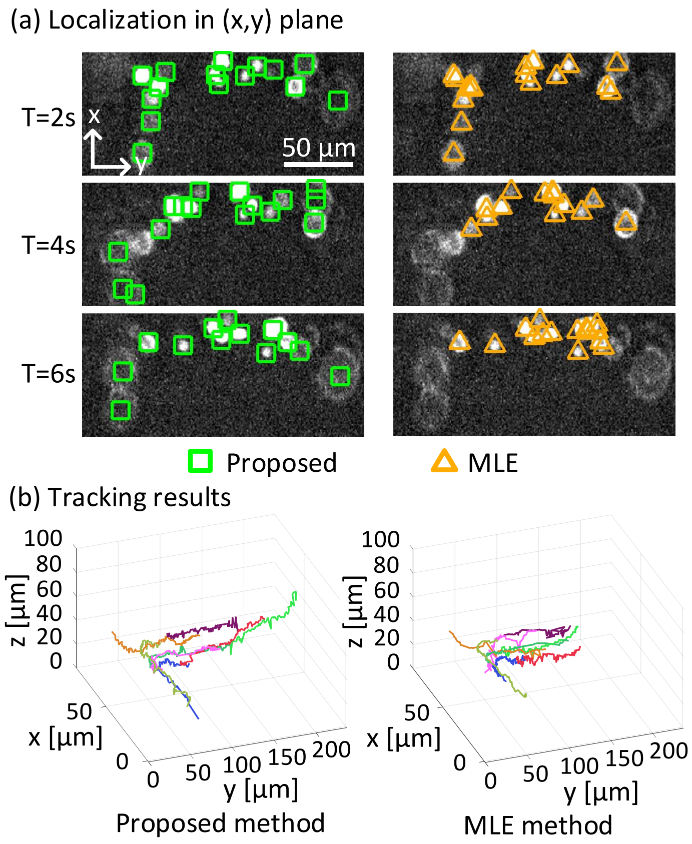


Figure 5: The 3D tracking of blood cells in a zebrafish. (a) The wide-field fluorescence images marked with the localization results by our method and the MLE method at different stamps. (b) The comparison of the tracking traces in 3D.

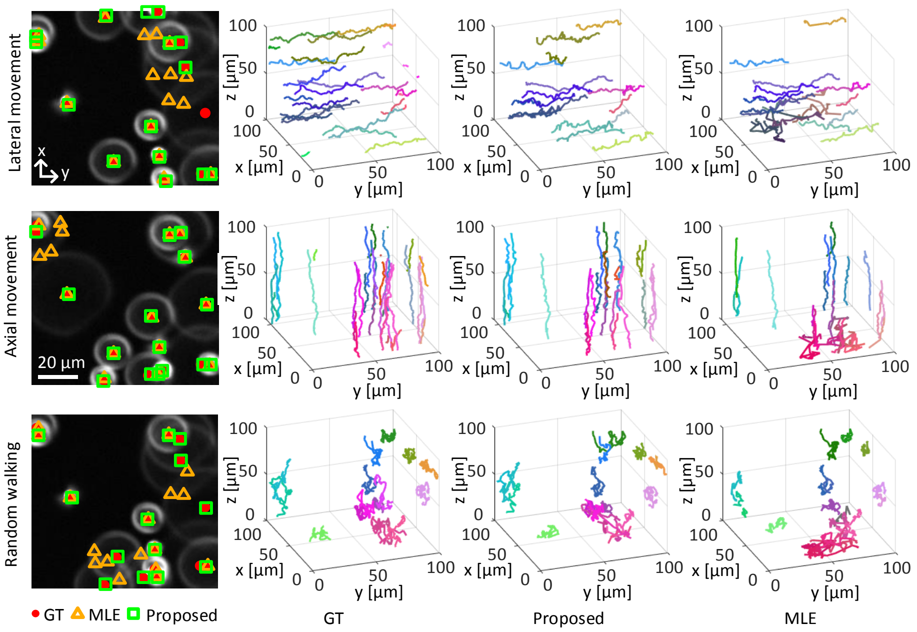


Figure 6: Simulated 3D tracking results for our method and MLE method with respect to different moving patterns: lateral movement, axial movement, and random walking. The first column illustrates localization results for one of the frames. The last three columns shows the 3D tracklets of GT, proposed method and MLE method respectively. (Different colors correspond to different beads.)
